# Supplementary material for: Evonne: Interactive Proof Visualization for Description Logics (System Description) -- Extended Version
Source: arXiv:2205.09583 source file (2022-05-19)
Supplement: Supplementary file 1 [file appendix-evonne.tex]

\subsection{Additional Details About the Graphical User Interface}

As mentioned earlier, the focus of this paper is on the proof component of \Evonne. For a general 
overview of the system, we show an example in Fig.~\ref{fig:evonne-overview} where both a proof 
and an ontology are presented in a split-view.

In the proof view of \Evonne, green vertices contain axioms 
of the ontology, blue ones contain inferred axioms, and the purple vertex contains the final conclusion.
In the bidirectional layout, axiom vertices are equipped with two sets of (\evUp,~\evDown) buttons 
located on their the top- and bottom-right corners.
Clicking the \emph{pull up} button (\evUp~top corner) of a node $n$, reveals a new inference in which
$n$ is a premise. Revealing an inference with conclusion $n$ can be achieved 
by clicking its \emph{pull down} button (\evDown~bottom corner).
Fig.~\ref{fig:magic-a} depicts the effect of pulling up, Fig.~\ref{fig:magic-c} depicts the effect of 
pulling down.
Analogously, clicking the \emph{push down} button (\evDown~top corner) of a node $n$ hides the 
inference that has $n$ as a conclusion. Hiding an inference with premise $n$
can be achieved by clicking its \emph{push up} button (\evUp~bottom corner).
The effect of pushing is shown in Fig.~\ref{fig:magic-b}.
In general, pull and push functionalities can lead to the generation of new magic nodes.

\begin{figure}[tb]
    \includegraphics[width=1\textwidth]{screenshots/overview-proof-ont.png}
    \caption{System overview}
    \label{fig:evonne-overview}
\end{figure}

\begin{figure}[tb]
    \includegraphics[width=1\textwidth]{screenshots/magic.png}
    \begingroup
    \phantomsubcaption\label{fig:magic-a}
    \phantomsubcaption\label{fig:magic-b}
    \phantomsubcaption\label{fig:magic-c}
    \endgroup
    \caption{Illustration of pulling and pushing \wrt magic inferences in \Evonne}
    \label{fig:magic}
\end{figure}
